# Supplementary material for: Multidimensional Perceptron for Efficient and Explainable Long Text Classification
Source: arXiv:2304.01638 source file (2023-04-04)
Supplement: Supplementary file 1 [file 8_Appendix.tex]

\section{Appendices}
